# Supplementary material for: MVTrans: Multi-View Perception of Transparent Objects
Source: arXiv:2302.11683 source file (2023-02-22)
Supplement: Supplementary file 1 [file appendix.tex]

%%%%%%%%%%%%%%%%%%%%%%%%%%%%%%%%%%%%%%%%%%%%%%%%%%%%%%%%%%%%%%%%%%%%%%%%%%%%%%%%
\section*{APPENDIX}

\subsection{Related Work}
\subsubsection{Transparent Object Depth Estimation}

Depth estimation refers to the task of predicting a dense depth map of a given scene. Recent advances of learning based depth estimation can be classified based on their expected inputs: monocular RGB image, monocular RGB-D image, stereo image pair, and multi-view images. 
Monocular RGB depth estimation refers to the direct regression of depth from RGB input \cite{eigen2014depth,ranftl2020robust,laina2016deeper,chen2017singleimage}. Convolutional neural networks (CNN) and recently, vision transformers\cite{monoDepthTransformer} are studied to explore its superior capability in depth regression compared to classical approaches. However, these methods are hindered by its single-view input constraints and the consequential scale ambiguity problem caused by one-point perspective from a image\cite{ESPDepth}.
RGB-D based depth estimation tasks aim to correct the incomplete or incorrect depth reported by sensors using color image and raw sensor depth. Some works demonstrate the effectiveness of a global optimization approach, which leverages the combination of predicted surface normal, occlusion boundary and original depth for depth estimation guidance \cite{ClearGrasp, rgbd_depth}.  Other methods use encoder-decoder or Generative Adversarial Networks (GANs) to generate the completed depth map by regression\cite{senushkin2021decoder, RGBDGAN}. 
Stereo image based depth estimation calculates depth via disparity prediction using stereo matching. Considering the difficulty of similarity estimation for traditional patch matching methods, recent methods apply learning based neural networks to improve disparity prediction accuracy \cite{DBLP:journals/corr/ZbontarL14, DBLP:journals/corr/abs-2103-03922}.
%Multi-view stereo based methods are closely related to stereo image, where instead of two images from a narrow baseline, multiple images from different viewing angles are considered and all of them are plane sweeping wrap \cite{planeSweep} into single matching cost volume. The merged cost volume is then used to generate the depth using 3D convolution \cite{MVSN, ESPDepth}.

Transparent objects introduce additional challenges in perception compared to common opaque objects. Namely, their reflective surface and transparent nature leads to changed appearances depending on viewing angle, and a distorted depth modality. Several papers have tackled the problem of transparent object depth estimation. ClearGrasp \cite{ClearGrasp} takes a global optimization based approach, using RGB-D as input and regresses the complete depth using predictions from individual models for surface normal, segmentation, and occlusion boundaries. Seeing Glass \cite{seeingGlass} uses two-stage joint point cloud and depth completion based method to predict the complete depth from noisy RGB-D.  \cite{zhu2021rgbd} proposed a voxel-based local implicit neural function for depth estimation using RGB-D. In contrast to previous RGB-D and multi-component methods, our approach uses multi-view RGB images as input and applies a fully end-to-end architecture for regression of several perception cues, including depth.

\subsubsection{Transparent Object Segmentation} % Allan
Transparent object segmentation is a common problem in computer vision and different robotic applications. Specifically, \cite{1467548, 1640865, https://doi.org/10.48550/arxiv.2003.13948, https://doi.org/10.48550/arxiv.2103.13279, DBLP:journals/corr/abs-2103-15734} aim to improve the performance of general object recognition and segmentation on particular transparent objects. \cite{DBLP:journals/corr/abs-2107-03172, https://doi.org/10.48550/arxiv.2003.13948, DBLP:journals/corr/abs-2103-15734,DBLP:journals/corr/abs-2101-08461} segment transparent and reflective surfaces for visual navigation and scene understanding. Several monocular RGB methods leverage the unique difference in appearance and texture along the edge of transparent vessels by incorporating boundary cues \cite{ https://doi.org/10.48550/arxiv.2003.13948, https://doi.org/10.48550/arxiv.2103.13279, DBLP:journals/corr/abs-2103-15734}. Recent methods encode image features using transformer blocks to leverage the attention mechanism and learn better global-context information for segmentation \cite{DBLP:journals/corr/abs-2107-03172, DBLP:journals/corr/abs-2101-08461}. In the robotics domain, transparent object segmentation is used as an auxiliary task to estimate the rough locations of objects on the image, which benefits downstream depth completion \cite{xu2021seeing} and object pose estimation \cite{sajjan2019cleargrasp, https://doi.org/10.48550/arxiv.2106.16118, DBLP:journals/corr/ZengYSSWRX16}.

\subsection{Transparent Object Depth Estimation}

Depth estimation refers to the task of predicting a dense depth map of a given scene. Recent advances of learning based depth estimation can be classified based on their expected inputs: monocular RGB image, monocular RGB-D image, stereo image pair, and multi-view images. 
Monocular RGB depth estimation refers to the direct regression of depth from RGB input \cite{eigen2014depth,ranftl2020robust,laina2016deeper,chen2017singleimage}. Convolutional neural networks (CNN) and recently, vision transformers\cite{monoDepthTransformer} are studied to explore its superior capability in depth regression compared to classical approaches. However, these methods are hindered by its single-view input constraints and the consequential scale ambiguity problem caused by one-point perspective from a image\cite{ESPDepth}.
RGB-D based depth estimation tasks aim to correct the incomplete or incorrect depth reported by sensors using color image and raw sensor depth. Some works demonstrate the effectiveness of a global optimization approach, which leverages the combination of predicted surface normal, occlusion boundary and original depth for depth estimation guidance \cite{ClearGrasp, rgbd_depth}.  Other methods use encoder-decoder or Generative Adversarial Networks (GANs) to generate the completed depth map by regression\cite{senushkin2021decoder, RGBDGAN}. 
Stereo image based depth estimation calculates depth via disparity prediction using stereo matching. Considering the difficulty of similarity estimation for traditional patch matching methods, recent methods apply learning based neural networks to improve disparity prediction accuracy \cite{DBLP:journals/corr/ZbontarL14, DBLP:journals/corr/abs-2103-03922}.

\subsection{Object Pose Estimation} % Helen / Allan

Object pose estimation predicts the 6-DoF pose of rigid objects. Typical methods concern either axis-aligned bounding box, or oriented bounding box. Some existing works use CNNs to train from either monocular color image input \cite{Xiang2018PoseCNNAC, Kehl2017SSD6DMR, CDPN, GDR-Net, dengsheng-pose, single-stage-6dpose}, or RGB-D input \cite{Wang2019DenseFusion6O,He2020PVN3DAD,Wada2020MoreFusionMR}. Keypoint-based approaches predict the eight vertices of the object's 3D bounding box \cite{Tekin2018RealTimeSS,Rad2017BB8AS, Tremblay2018DeepOP}, or predict points on the object surface \cite{Peng2019PVNetPV, Song2020HybridPose6O}. Dense 2D-3D correspondence methods first predict the point cloud of the object and then conduct association and pose computation by correspondence with a ground truth model or mapping \cite{Chen2020EndtoEndLG,Hodan2020EPOSE6,Park2019Pix2PosePC}. More recent works apply the concept of first detecting 2D targets and then solving a Perspective-n-Point (PnP) problem for the object pose which combines the idea of 2D-3D mapping and keypoints methods. For transparent object pose estimation, KeyPose is a stereo RGB and keypoint based method \cite{keypose}. SimNet is a stereo and oriented 3D BBox based method. And another method \cite{6dof-pose},  incorporates a two-stage approach, using predicted segmentation, surface normal, and plane to perform pose estimation.

\section{annotation}
\textbf{2D \& 3D Bounding Box.} The 2D bounding box coordinates in the image frame are provided for all objects. The vertices for the 3D Bounding Box are provided in image frame, local frame, and camera frame. \\
% \textbf{3D Bounding Box.} \\
\textbf{Object Pose.} Object pose is provided in two means: homogeneous transformation matrix from local frame to camera frame, and covariance matrix based on the transformed point cloud in the camera frame. \\
\textbf{Keypoints.} Eight keypoints are sampled using the Furthest Point Sampling (FPS) algorithm. The keypoints are given in the local frame, and can be transformed to the camera frame using the local to camera frame transformation matrix. \\
\textbf{Segmentation.} For each object, the full and visible segmentation are provided. Full segmentation ignores any occlusion, and masks the full object regardless of occlusion. Visible segmentation only shows the non-occluded regions of objects.\\
\textbf{Depth and Tangent Normals.} The ground truth depth is provided in metres, and tangent space normal of the entire view is provided as captured in the camera frame. \\ 
\textbf{Heatmaps. } Gaussian heatmap centered at the centroid of each rigid object within the camera view, with variance determined by the associated visible segmentation map.
